# Supplementary material for: Terahertz tuning of Dirac plasmons in Bi$_2$Se$_3$ Topological Insulator
Source: arXiv:1910.11233 source file (2019-10-24)
Supplement: Supplementary file 1 [file SupplementalMaterial.pdf]

# Supplemental Material of the article:

# Terahertz tuning of Dirac plasmons in $Bi_2Se_3$ Topological Insulator

## Part 1: Extinction coefficient

The extinction coefficient data reported in Fig. 2 of the main manuscript have been measured for both samples with the experimental set-up described in Fig 5 of Ref [1]. By employing a step-scan Michelson interferometer and a He-cooled bolometer as a detector, we measured the transmitted THz intensity $I_S(\nu)$ of $Bi_2Se_3$ patterned thin films (with 4 and 20 μm of ribbon width, respectively), deposited on sapphire (500 microns thick) substrate with respect to the background intensity $I_0(\nu)$. The transmittance $T(\nu)= I_S(\nu)/I_0(\nu)$ has been measured for each value of the incident THz electric field, which has been varied through two crossed polarizers mounted before the sample (see Fig 5 of Ref [1]). A third polarizer is located in front of the sample in order to select the right polarization for exciting the plasmon (polarization perpendicular to the ribbons) or the Drude term (polarization parallel to the ribbons). From the transmittance $T(\nu)$ we calculated the extinction coefficient by the formula:

$$E(\nu) = 1 - T(\nu) \qquad \text{(S1)}$$

The final data are those reported in Fig. 2 (open circles) of the main manuscript.

## Part 2: Fitting procedure: Fano model

The presence of Dirac plasmon absorption in the ribbon array samples close to the main IR phonon of $Bi_2Se_3$ (centered at nearly 2 THz) leads to a Fano interaction between them (Ref. [2]). The Fano interaction between the two modes causes a hardening of the mode at higher frequencies and a softening of the mode at lower frequencies. Hence, in order to extract the bare frequency of the Dirac plasmon ($\nu_p$) for every value of the incoming THz electric field, we fitted the extinction coefficient by the same model used in Ref. [2] and described in detail in Ref. [3]. The fitting equations are:

$$E(\nu') = \frac{(\nu' + q(\nu'))^2}{\nu'^2 + 1} \frac{g^2}{1 + \left(\frac{\nu - \nu_p}{\Gamma_p/2}\right)^2} \qquad \text{(S2)}$$

$$\nu' = \frac{\nu - \nu_{ph}}{\Gamma_{ph}(\nu)/2} - \frac{\nu - \nu_p}{\Gamma_p/2} \qquad \text{(S3)}$$

$$q(\nu) = \frac{\nu w/g}{\Gamma_{ph}(\nu)/2} \frac{\nu - \nu_p}{\Gamma_p/2} \qquad \text{(S4)}$$

The plasmon-coupled phonon linewidth can be separately calculated by the expression:

$$\Gamma_{ph}(\nu) = \frac{2\pi v^2}{1 + \left(\frac{\nu - \nu_p}{\Gamma_p/2}\right)^2} \qquad \text{(S5)}$$

According to Eq. (S2-S5), one has six free fitting parameters g, w, v, $\nu_p$, $\Gamma_p$ and $\nu_{ph}$. However, one of these parameters is constrained, being $g = \Gamma_p^{1/2}$ (Ref. [3]). Moreover, $\nu_{ph}$ is known from independent measurements of parallel polarization spectra. Therefore, the free fit parameters of the fluence dependent extinction coefficients are actually four. In Tables 1, 2 we report all of them *vs.* the incoming THz electric field.

| $E_{THz}$ (kV/cm) | $\nu_p$ (THz) | $\Gamma_p$ (THz) | $\nu_{ph}$ (THz) | g ($THz^{1/2}$) | w (THz) | v ($THz^{1/2}$) |
|---|---|---|---|---|---|---|
| 0.1 | 1.80 | 1.20 | 1.90 | 1.10 | 0.2850 | 0.364 |
| 99 | 1.80 | 1.48 | 1.89 | 1.22 | 0.0285 | 0.399 |
| 283 | 1.77 | 1.42 | 1.86 | 1.19 | 0.0322 | 0.328 |
| 518 | 1.74 | 1.38 | 1.88 | 1.18 | 0.0881 | 0.515 |
| 1000 | 1.64 | 1.52 | 1.92 | 1.23 | 0.0464 | 0.515 |

Table S1: Fitting parameters of the 4 μm ribbon width sample *vs.* the incoming electric field.

| $E_{THz}$ (kV/cm) | $\nu_p$ (THz) | $\Gamma_p$ (THz) | $\nu_{ph}$ (THz) | g ($THz^{1/2}$) | w (THz) | v ($THz^{1/2}$) |
|---|---|---|---|---|---|---|
| 0.1 | 1.50 | 0.845 | 1.79 | 0.919 | 0.300 | 0.348 |
| 110 | 1.50 | 0.991 | 1.77 | 0.995 | 0.030 | 0.222 |
| 570 | 1.37 | 1.310 | 1.77 | 1.150 | 0.265 | 0.288 |
| 1200 | 0.90 | 0.646 | 1.73 | 0.804 | 0.024 | 0.555 |

Table S2: Fitting parameters of the 20 μm ribbon width sample *vs.* the incoming electric field.

## Part 3: Plasmon softening: comparison with theoretical models

In Fig. 3 of the main manuscript we report the bare plasmon frequency $\nu_p$ for both samples (2$^{nd}$ column of Tables S1, S2), with respect to the THz electric field (1$^{st}$ column in Tables S1, S2). These experimental data are compared to theoretical calculations in the main manuscript (see Fig 3) which are discussed in the following sections.

### Sommerfeld expansion

The plasmon frequency is proportional to the chemical potential of the Dirac fermion gas (Ref. [4])

As the chemical potential ($\mu$(T)) depends on temperature (T) through the Sommerfeld expansion, one can finally estimate the plasmon frequency *vs.* T through the following equations (Ref. [4-5]):

$$\mu(\mathrm{T}) \cong \mathcal{E}_F\left(1-\frac{\pi^2 k_B^2 T^2}{6\varepsilon_F^2}\right) \qquad \text{(S6)}$$

$$\nu_P(\mathrm{T}) \cong \nu_P(\mathrm{T}=0)\left(1-\frac{\pi^2 k_B^2 T^2}{6\varepsilon_F^2}\right)^{1/2} \qquad \text{(S7)}$$

where the Fermi energy, $\mathcal{E}_F$ (the chemical potential at zero temperature), is the only intrinsic parameter characterizing the Dirac fermion gas. $\mathcal{E}_F$ as estimated from transport and optical properties of the material is nearly 230 meV.

The 1$^{st}$ order Sommerfeld expansion in (S7) can be further compared with a numerical calculation of the temperature-dependence of the chemical potential. As already done in Ref. [5], we calculate μ(T) by imposing charge conservation at different temperatures, through

$$n=\int_{-\infty}^{\infty}\frac{g(E)dE}{1+\exp\left[\frac{E-\mu(T)}{k_B T}\right]} \qquad \text{(S8)}$$

The comparison between the 1st order Sommerfeld approximation and the numerical calculation is reported in Fig. S1. In the temperature range considered here, the deviations of the chemical potential between the two models is within 9%. This yields a difference in terms of estimated plasmon frequency which is below 3%, well below our experimental uncertainty.

It shows that the deviation of the 1st order Sommerfeld approximation from the numerical calculation in the range of the THz electric field here investigated is of about 3%. For that reason we extracted the experimental electronic temperature (reported in Fig. S3 as a function of the THz electric field) from Eq. S7, by using the relation between the electronic temperature and the pump field given by the Two-temperature model, described below.

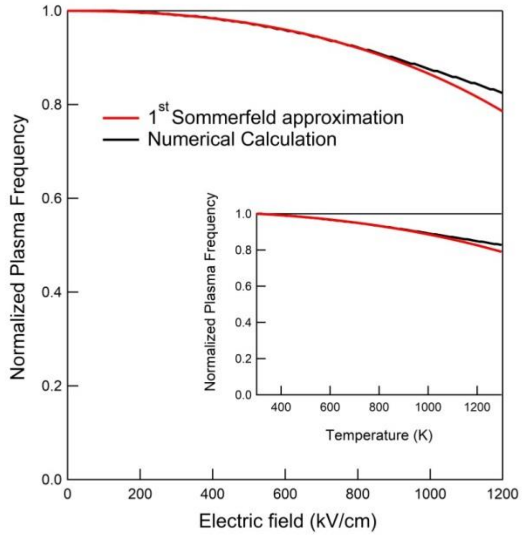


Fig. S1: Evolution of the normalized plasmon frequency *vs* the THz electric field within the 1st order Sommerfeld approximation (Eq. S7) and from the numerical calculation (see text). For the sake of comparison, the inset shows also the two calculations as a function of temperature in the range of electronic temperatures reached in our experiment. The temperature dependence has been converted into the THz electric field dependence, by using the "Two-temperature" model described in the text (next session).

## Thermodynamic model: "Two-temperature" model

Equations 3-4 in the main text describe the evolution of electronic and the lattice temperatures in a material absorbing a pump beam and are reported here below (Eq. S8 and S9). In particular, the theoretical electronic $T_e$ and lattice $T_l$ temperatures have been calculated by using the microscopic parameters listed below. In Fig S2 we show the temporal trend of both temperatures.

$$c_e(T_e)\frac{dT_e}{dt} = -G(T_e)(T_e - T_l) + \mathrm{P(t)} \qquad \text{(S8)}$$

$$c_l(T_e)\frac{dT_l}{dt} = G(T_e)(T_e - T_l) \qquad \text{(S9)}$$

Where $c_e(T_e)$ and $c_l(T_e)$ are the electronic and lattice specific heat, respectively. $G(T_e)$ is the coupling parameter between the electron and the phonon subsystems. Here below we report the microscopic parameters $c_e$, $c_l$, $G$ and the THz pump power $P(t)$ absorbed by the samples, that have been used for solving Eq. S8-S9:

- $c_e = \gamma_e T_e$ where $\gamma_e = \frac{2\pi k_B^2 E_F}{3\hbar^2 v_F^2} = 3.7 \times 10^{-9}$ $JK^{-2}m^{-2}$, with $E_F = 230$ meV and $v_F = 6 \times 10^5$ m/s
- $G = \gamma_{e\text{-}ph} c_e$ where $\gamma_{e-ph} = \frac{3\lambda E_{ph}^2}{\pi\hbar k_B} = 1.1 \times 10^{15}\ s^{-1}$, with $\lambda = 0.25$ (Ref [7]) and $E_{ph} = 15.9$ meV (Debye phonon energy)
- $c_l = 2.81 \times 10^{19}\, k_B \left(\frac{k_B T_L}{E_{ph}}\right)^3 \int_0^{\frac{E_{ph}}{k_B T_L}} \frac{x^4 e^x}{(e^x-1)^2} dx$ (Ref. [8])
- $P(t) = A\ F\ g(t)$, where A is the absorption coefficient calculated from optical properties in parallel polarization (see next section), considering the thickness of the sample (d=60 nm) and the patterning filling factor (0.5).

  F is the fluence of the pump and g(t) is a normalized gaussian function that well reproduces the shape of the incoming THz pulse with a variance $\sigma_t$ of 0.33 ps (~ 0.8 ps FWHM), that is

$$g(t) = \frac{1}{\sigma_t\sqrt{2\pi}} \exp\left(-\frac{1}{2}\left(\frac{t-t_0}{\sigma_t}\right)^2\right)$$

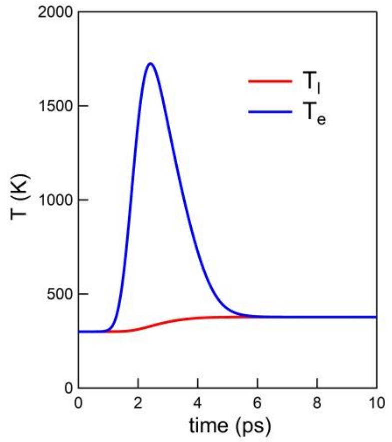


Fig. S2: Temporal evolution of the electronic temperature ($T_e$) and the lattice temperature ($T_l$) from the theoretical "Two-temperature" model (see main manuscript).

In Fig S3 we compare the experimental electronic temperatures for both samples and the theoretical electronic temperature as a function of the pump fluence. The experimental electronic temperature has been extracted from the Sommerfeld expansion (Fig. S1) by inverting Eq. S7. The theoretical electronic temperature (dashed green curve in Fig. S3) have been calculated by convolving $T_e$ with the temporal evolution of the pump for every value of the fluence.

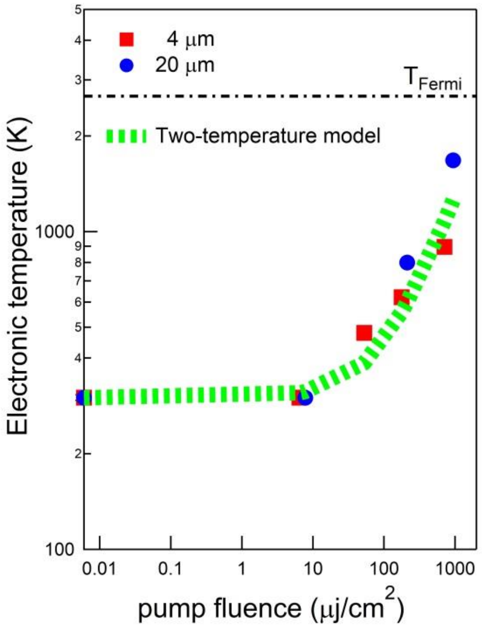


Fig. S3: Experimental electronic temperatures of the two samples (blue and red points), compared with the theoretical temperatures calculated by the "Two-temperature" model (dashed green line). The pink dots derived from time-resolved ARPES experiments, reported in Ref. [9-10]. The black dashed line is the Fermi temperature of the present $Bi_2Se_3$ films, equal to 2670 K.

## Representative spectrum of the source

A representative spectrum of the source at the TeraFERMI beamline (see Ref. [1]) during the experiment is reported in Fig. S3. It was acquired by means of the same experimental set-up used for measuring the sample spectra, by simply removing the sample from the focus position.

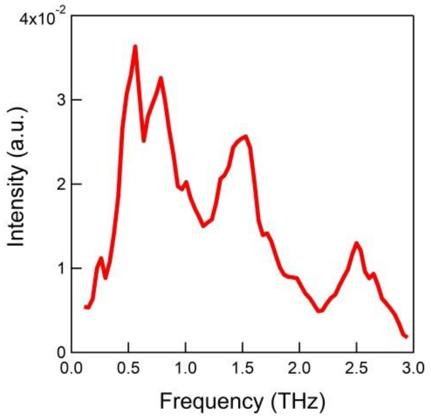


Fig. S3: Representative spectrum of the THz source during the experiment.

## Parallel polarization: extraction of optical conductivity

The 20 μm ribbon sample has been measured also for light parallelly polarized with respect to the ribbons. In this case, superimposed to the main IR active phonon at about 2 THz, only the Drude response can be detected. From transmittance data, measured as a function of fluence, one can extract the optical conductivity, using the formula for thin films that provides the real part of the conductance $\sigma_{\square}$ (in thin film approximation) (Ref. [9])

$$\sigma_{\square} = \left(\frac{n+1}{Z}\right)\left(\frac{1}{\sqrt{T}} - 1\right) \qquad \text{(S9)}$$

where n is the refractive index of the substrate (in our case, sapphire, *i.e.* n=10.5) and Z is the vacuum impedance equal to 377 Ω. From the conductance, we can easily calculate the real part of the optical conductivity by:

$$\sigma = \frac{\sigma_{\square}}{d} \qquad \text{(S10)}$$

where d is the thickness of the sample, equal to 60 nm. In Fig. S4 we show the optical conductivities in non-linear regime, for two different value of the electric field, calculated by Eq. (9-10). One can observe that, like in the case of graphene shown in Ref. [5], the Drude weight of optical conductivity decreases as the incoming THz electric field increases.

These data have been fitted to a Drude-Lorentz model,

$$\sigma = \frac{1}{4\pi}\left(\frac{{\nu_D}^2\ \Gamma_D}{\nu^2+(\Gamma_D/2\pi)^2} + \frac{{W_{ph}}^2\ \nu^2\Gamma_{ph}}{(\nu^2-\nu_{ph}^2)^2+(\Gamma_{ph}\nu/2\pi)^2}\right) \qquad \text{(S11)}$$

where $\nu_D$ and $\Gamma_D$ are the Drude weigth and its scattering rate, respectively, while $W_{ph}$, $\nu_{ph}$, $\Gamma_{ph}$ are the oscillator strength, the phonon frequency and its scattering rate, respectively.

All optical fitting parameters are reported in Table S3. Since the fitted data related to patterned samples, it is worth to notice that one has to take into account the filling factor 0.5 to recover the actual properties of the material.

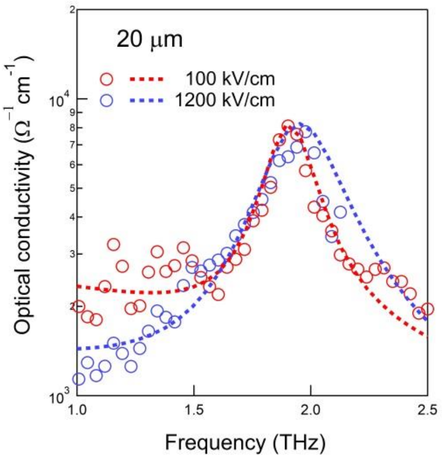


Fig. S4: Optical conductivities of 20 μm sample in parallel polarization. Here we compared data between two different incoming THz electric fields.

| Parameters (THz) | $E_{THz}$ = 100 kV/cm | $E_{THz}$ = 1200 kV/cm |
|---|---|---|
| $\nu_D$ | 17 | 13 |
| $\Gamma_D$ | 2.3 | 2.4 |
| $W_{ph}$ | 55 | 73 |
| $\nu_{ph}$ | 1.9 | 2.0 |
| $\Gamma_{ph}$ | 0.24 | 0.39 |

Table S3: Drude-Lorentz fitting parameters of the optical conductivities for three different values of the THz electric field for the sample with ribbon width 20 μm, reported in Fig. S5. The parameters are those related to Eq. S12.

## Non-perturbative Boltzmann model

A non-perturbative approach to the kinetic Boltzmann equation in the case of graphene, was provided in Ref. [6], while the resulting softening of plasmon excitation in the presence of strong THz pulses in a ribbon film was presented in Ref. [7]. According to these references, the linear (intraband) conductivity

$$\sigma(\nu) = \frac{e^2 \epsilon_F}{\pi \hbar^2} \frac{i}{2\pi\nu + {}^{i}/_{\tau}} \qquad \text{(S12)}$$

should be replaced in the non-linear regime by the formula

$$\sigma_{\nu,\nu}(\nu\tau, \mathcal{F}_\tau) = \sigma_0 S_1(\nu\tau, \mathcal{F}_\tau) \qquad \text{(S13)}$$

where $\sigma_0$ is the static conductivity and

$$\mathcal{F}_\tau = \frac{e E_{THz} \tau}{\hbar k_F} \qquad \text{(S14)}$$

is a dimensionless field parameter already introduced in the main text, while

$$S_1(\nu\tau, \mathcal{F}_\tau) = \int_0^\infty e^{-\xi} \frac{\sin(\pi\nu\tau\zeta)}{\pi\nu\tau\zeta} B_1\left(\mathcal{F}_\tau \frac{\sin(\pi\nu\tau\zeta)}{\pi\nu\tau\zeta}\right) e^{i\pi\nu\tau\xi} d\xi \qquad \text{(S15)}$$

with

$$B_1(a) = \frac{4}{\pi} \int_0^{\pi/2} \frac{sin^2 x}{\sqrt{1+(a\sin x)^2}} \ {}_2F_1(\frac{1}{4}, \frac{3}{4}, 2; (\frac{2a\sin x}{1+(a\sin x)^2})^2) dx \qquad \text{(S16)}$$

${}_2F_1(a,b,c;x)$ being the hypergeometric function.

The plasmon dispersion relation can be determined from the following Equation

$$\epsilon_{nonlin}(q, \nu) \equiv 1 + \frac{i}{\nu\bar{\epsilon}} \frac{e^2}{\pi\hbar} \frac{\epsilon_F \tau}{\hbar} S_1(\nu\tau, \mathcal{F}_\tau) q = 0 \qquad \text{(S17)}$$

$$\Rightarrow 1 + i(2\pi\nu_p\tau)^2 \frac{S_1(\nu\tau, \mathcal{F}_\tau)}{2\pi\nu\tau} = 0 \qquad \text{(S18)}$$

where $\bar{\epsilon}$ is the effective dielectric constant, as already introduced in the main text, and $\nu_p = \left(\frac{e^2 \epsilon_F}{\pi\hbar^2\bar{\epsilon}} q\right)^{1/2}$ is the usual plasmon frequency, as found in the linear regime. The non-linear optical absorption can then be written in the form:

$$A_{nonlin}(\nu) \propto \frac{S_1(\nu\tau, \mathcal{F}_\tau)}{\left|1 + i(2\pi\nu_p\tau)^2 S_1(\nu\tau, \mathcal{F}_\tau)/2\pi\nu\tau\right|^2} \qquad \text{(S19)}$$

The non-linear plasmon frequency $\nu_p^{nonlin}$ is found by calculating the value of $\nu$ which maximizes $A_{nonlin}(\nu)$.

## References


[1] Di Pietro, P. et al. *Synchrotron radiation News* **30,** 36-39 (2017).

[2] Di Pietro P. et al. *Nature Nanotechnology* **8**, 556 (2013).

[3] Giannini, V. et al. *Nano Letters* **11**, 2835-2840 (2011).

[4] Jadidi, M. M. et al. *Nano Letters* **16**, 2734 (2016).

[5] Mics, Z. et al. *Nature Communications* **6**, 7655 (2015).

[6] Mikhailov, S. A. *Phys. Rev. B* **95**, 085432 (2017).

[7] Mikhailov, S. A. *ACS Photonics* **4**, 3018-3022 (2017).

[8] Lai, Y.-P. et al. *Appl. Phy. Lett.* **105**, 232110 (2014).

[9] Henning, P. F. et al. *Phys. Rev. Lett.* **83**, 23 (1999).
